# Supplementary material for: Summarizing long regulatory documents with a multi-step pipeline
Source: arXiv:2408.09777 source file (2024-10-14)
Supplement: Supplementary file 1 [file Human_evaluation_document_answers_only_appendix.pdf]

# Summary 1

## *Participant 1:*

### Metric Ratings

1. Factual Correctness: 1
2. Usability: 1
3. Accuracy: 1
4. Fluency: 1
5. Coherence: 1

### Additional Feedback:

This summary would not be usable, because if someone that has no knowledge in the topic would read this, they would not understand a thing about the actual regulation, due to the incompleteness, occurrence of factual mistakes and inaccuracy.

## *Participant 2:*

### Metric Ratings

1. Factual Correctness: [1-5] → 3
2. Usability: [1-5] → 3
3. Accuracy: [1-5] → 2
4. Fluency: [1-5] → 2
5. Coherence: [1-5] → 3

### Additional Feedback:

[Your comments]
Touches upon main principle of CBAM, but some of the procedures/rules are described incorrectly.

## Summary 2

### *Participant 1:*

#### Metric Ratings

1. Factual Correctness: 3
2. Usability: 1
3. Accuracy: 1
4. Fluency: 2
5. Coherence: 1

#### Additional Feedback:

Summary does not per se contain false information, however it misplaces information (in a false manner). For example: in the ‘key points’ it describes background information of the regulation instead of the main content of the regulation. This summary would not be usable for readers.

### *Participant 2:*

#### Metric Ratings

1. Factual Correctness: [1-5] → 4
2. Usability: [1-5] → 1
3. Accuracy: [1-5] → 3
4. Fluency: [1-5] → 4
5. Coherence: [1-5] → 2

#### Additional Feedback:

[Your comments]
The summary completely misses out on the main point of what CBAM is.
State information appears to be correct (few mistakes).

## Summary 3

### *Participant 1:*

#### Metric Ratings

1. Factual Correctness: 4
2. Usability: 3
3. Accuracy: 3
4. Fluency: 2
5. Coherence: 2

#### Additional Feedback:

This summary is actually quite useful: it correctly grasps the key points of the regulation. It is not fully complete, and the fluency and coherence of the sentences are a bit lacking, but this summary is a good starting point.

### *Participant 2:*

#### Metric Ratings

1. Factual Correctness: [1-5] → 4
2. Usability: [1-5] → 4
3. Accuracy: [1-5] → 3
4. Fluency: [1-5] → 4
5. Coherence: [1-5] → 4

#### Additional Feedback:

[Your comments]

## Summary 4

### *Participant 1:*

#### Metric Ratings

1. Factual Correctness: 1
2. Usability: 1
3. Accuracy: 1
4. Fluency: 1
5. Coherence: 1

#### Additional Feedback:

This summary is less bad than Summary 1, but still unusable as it contains a lot of false information/incorrect words.

### *Participant 2:*

#### Metric Ratings

1. Factual Correctness: [1-5] → 3
2. Usability: [1-5] → 3
3. Accuracy: [1-5] → 4
4. Fluency: [1-5] → 2
5. Coherence: [1-5] → 3

#### Additional Feedback:

[Your comments]

## Summary 5:

## *Participant 1:*

### Metric Ratings

1. Factual Correctness: 4
2. Usability: 1
3. Accuracy: 2
4. Fluency: 1
5. Coherence: 1

### Additional Feedback:

The summary started really well, however it started repeating the same sentence over and over at some point. Therefore not usable.

## *Participant 2:*

### Metric Ratings

1. Factual Correctness: [1-5] → 3
2. Usability: [1-5] → 1
3. Accuracy: [1-5] → 3
4. Fluency: [1-5] → 5
5. Coherence: [1-5] → 1

### Additional Feedback:

[Your comments]
A lot of repetition

## Summary 6:

### *Participant 1:*

#### Metric Ratings

1. Factual Correctness: 3
2. Usability: 1
3. Accuracy: 2
4. Fluency: 1
5. Coherence: 1

#### Additional Feedback:

Again unusable due to the sentences that are repeated. However, some of the sentences that are not repeated contain quite some useful information.

### *Participant 2:*

#### Metric Ratings

1. Factual Correctness: [1-5] → 3
2. Usability: [1-5] → 4
3. Accuracy: [1-5] → 3
4. Fluency: [1-5] → 4
5. Coherence: [1-5] → 3 (malus for repetition at end, otherwise 4)

#### Additional Feedback:

[Your comments]
